# Supplementary material for: LLMTreeRec: Unleashing the Power of Large Language Models for Cold-Start Recommendations
Source: arXiv:2404.00702 source file (2024-12-24)
Supplement: Supplementary file 1 [file 8Appendix.tex]

% \section{Experimental Details}

% \subsection{Datasets} \label{data}

% \begin{itemize}[leftmargin=*]
% % \item \textbf{MIND\footnote{https://msnews.github.io/}} is a large-scale news recommendation dataset collected from Microsoft News. It includes the historical behaviors of click and non-click on English news articles from a million users.
% \item 
% \textbf{MIND\footnote{https://msnews.github.io/}} is a large-scale dataset designed for research in news recommendation. It is compiled from anonymous behavioral logs on the Microsoft News website. The dataset comprises approximately 160,000 English news articles and 15 million impression logs generated by one million users. Each news article in MIND is enriched with extensive textual content, including titles, summaries, main text, categories, and entity information. Each impression log contains user click events, non-click events, and the user's historical news click behavior leading up to that impression. Considering user privacy protection, each user is anonymized through secure hashing before being dissociated from the production system. In the MIND dataset, each item is characterized by category and subcategory features. As a result, the items can be organized into a two-level item tree, with all items assigned to its corresponding leaf node located at the same level.

% \item
% % \textbf{Amazon-Review\footnote{https://cseweb.ucsd.edu/~jmcauley/datasets.html}} dataset is crawled from Amazon e-commerce platform containing not only the reviews and ratings from users but also the product information like price and category.
% \textbf{The Amazon-Review\footnote{https://cseweb.ucsd.edu/~jmcauley/datasets.html}} dataset is crawled from Amazon e-commerce platform containing not only the reviews and ratings from users but also the product information like price and category. In addition to the traditional features, it provides a the detail of user sentiments through textual feedback and the helpfulness ratings associated with each review. The dataset's richness is further enhanced by the link graphs illustrating item relationships, including the "also viewed" and "also bought" connections. We use the Movies and TV category within this dataset, which has 8,765,568 reviews and metadata for 203,970 distinct products. Notably, the Movies and TV dataset's metadata documents various hierarchical category information in a list format for each item. Leveraging this information, UniLLMRec has the capability to construct the item tree, offering semantic information for the language model to perform tree search.

% \end{itemize}
% Besides, for user-item interaction sequences, we limited their length to 50. Handling the extensive item subsets from some leaf nodes posed challenges for direct input into the Language Model (LLM) using a single prompt template. Consequently, we constrained each subset to a maximum of 50 items. Positive items were grouped into their respective subsets, and negative sampling was applied to each leaf node until reaching a size of 50. This process resulted in a candidate set of 1217 items for MIND and 6176 items for Amazon.

% \section{Baseline introduction}
% \item \textbf{Popularity-based recommendation} is a straightforward approach that ranks items based on their overall popularity among users, suggesting the most commonly chosen items.

% \item \textbf{Category-based popularity model} serves as a baseline by retrieving items through random sampling from each leaf node in the item tree, aligning with the popularity of semantic information in the user's interaction history.

% \item \textbf{FM}~\cite{rendle2010factorization} is a classic recommendation model enhancing system effectiveness through feature interactions.

% \item \textbf{DeepFM} \cite{guo2017deepfm} integrates FM (Factorization Machine) and DNN (Deep Neural Network) models, extracting low-order and high-order features for recommendations, making it a prominent recommendation model.

% \item \textbf{NRMS} \cite{wu2019neural} is a news recommendation model, which leverages multi-head self-attention and additive attention in the news and user encoder.

% \item \textbf{SASRec}~\cite{kang2018self} is a powerful sequential recommendation model with self-attention mechanism.

% \item \textbf{LLM-Ranker}~\cite{hou2024large} employs an LLM to rank an item list based on a candidate set. In the experiments, a random sampling approach is utilized to generate a prompt capable of accommodating as many items as possible.

% \subsection{Baseline implementation details}
% \label{appendix_baseline}
% For popularity-based models, we recall the top 20 items with the highest historical click-through rates based on user click history. Unfortunately, none of these 20 items were successfully recalled within the 500 samples selected for evaluation. Therefore, we conducted experiments on the entire test set, and the results are reported in Figure~\ref{fig8:Comparison_Recall_NDCG}. The FM, DeepFM, NRMS, and SASRec models all adopt a dual-tower structure, utilizing the Adam optimizer. Cross entropy is employed as the loss function, with a negative sampling ratio of 1 across all models. In the MIND dataset, all models use the item title as the input feature. However, in the Amazon dataset, using only the title feature leads to suboptimal performance for FM, DeepFM, NRMS, and SASRec. Consequently, for the Amazon dataset, we substitute the item description feature for the title as the input. For the DeepFM model, we set the embedding dimension to 50. In NRMS and SASRec, the embedding dimension is set to 300, with a dropout rate of 0.2.









%We utilize recall and NDCG metrics to assess the model's performance in recall tasks and employ ILAD~\cite{zhang2008avoiding} to evaluate the influence of re-ranking on diversity. 

\section{Case in MIND Dataset}
A case of \name(GPT-3.5) is shown here. The ground truth of this case is 
\begin{itemize}
    \item Some believe Mason Rudolph, hit in head with his own helmet, isn't getting enough blame
    \item Opinion: NFL should suspend Browns' Myles Garrett for rest of season   at minimum   for helmet swing
    \item This was uglier than a brawl. And Myles Garrett deserves suspension for rest of year after helmet attack.
\end{itemize}

The ground truth item is colored in red and the detailed case log is shown as follows:

\begin{tcolorbox}[%`colback`=gray!10,
            colframe=gray,
            width=1\linewidth,
            arc=1mm, 
            auto outer arc,
            title={User Profile Modeling},
            breakable,]
            \textbf{Input:}
            A user's click news are:\\
            Patrick Day in coma after suffering brutal knockout\\
            Cincinnati Bengals claim offensive lineman Fred Johnson\\
            High school soccer: Chloe DeLyser sets record for most goals scored\\
            Contractor claims video shows structural flaws prior to Hard Rock \\Hotel collapse\\
            Bengals release RB Samaje Perine, per report\\
            Winless Bengals bench Andy Dalton for rookie QB\\
            'When I smelled that smoke ... here we go again': Weary Californians \\seek shelter amid latest wildfire outbreak\\
            Obama calls out call-out culture: "That's not activism"\\
            The world's largest nuclear power producer is melting down\\
            Former NBA first-round pick Jim Farmer arrested in sex sting operation
            Bengals News (10/31): Rough deadline drama\\
            Joe Flacco to miss four to six weeks with neck injury\\
            DOJ sues Walmart for allegedly discriminating against a Navy reserve officer\\
            Cleveland Casino, Thistledown Sold: This Week's Must Read Stories
            Best Ski Resorts in the US\\
            Cause determined in Jessi Combs' fatal speed record crash\\
            New Mexico game vs. Air Force rescheduled after lineman Nahje \\Flowers' death\\
            How the Panthers will approach their breakup with Cam Newton before 2020 season\\
            Summarize the interested news topic categories, from the most important to the least important.

            
            \textbf{LLM:} Based on the provided news articles, the interested news topic categories can be summarized as follows, from the most important to the least important:

1. Sports: This category includes news about various sports events, such as boxing (Patrick Day's coma), football (Cincinnati Bengals signings and releases, Joe Flacco's injury), high school soccer records, and NBA player arrests.

2. Natural Disasters: This category includes news about wildfires in California and the collapse of the Hard Rock Hotel due to structural flaws.

3. Social Issues: This category includes news about former President Obama's criticism of call-out culture and the Department of Justice suing Walmart for alleged discrimination.

4. Nuclear Power: This category includes news about the world's largest nuclear power producer facing a meltdown.

5. Miscellaneous: This category includes news about the sale of a casino, the rescheduling of a football game after a player's death, and the breakup between the Carolina Panthers and Cam Newton.

6. Travel and Leisure: This category includes news about the best ski resorts in the US.

It's important to note that the importance of news topics can vary depending on individual interests and perspectives.
\end{tcolorbox}

\begin{tcolorbox}[%`colback`=gray!10,
            colframe=gray,
            width=1\linewidth,
            arc=1mm, 
            auto outer arc,
            title={Item Tree Search},
            breakable,]
            \textbf{Input:}
            Rank some topic categories from the following candidates to recommend to the user based on interests, from the most important to the least important without explanation:video,movies,foodanddrink,tv,finance,autos,entertainment,lifestyle,sports,weather,music,health,news,travel.

            \textbf{LLM:} Based on the limited information provided, the recommended topic categories for the user, from the most important to the least important, are as follows:

1. Sports

2. Entertainment

3. News

4. Travel

5. Music

6. Movies

7. Food and Drink

8. TV

9. Autos

10. Finance

11. Lifestyle

12. Health

13. Weather

14. Video

Please note that these recommendations are based solely on the given list of topic categories and may not reflect the user's specific interests.

\textbf{Input:} Provide a ranked list of top 10 subcategories based on the user's interest, without offering any explanations. Format your answer as follows: \{1. First Subcategory, 2. Second Subcategory, 3. Third Subcategory, ...\}.Here is the category and subcategory list:
football\_ncaa, tennis, baseball\_mlb\_videos, soccer, basketball\_nba, outdoors, football\_nfl, football\_nfl\_videos, icehockey\_nhl, more\_sports, baseball\_mlb, golf, soccer\_epl, basketball\_ncaavideo, entertainment-celebrity, humor, entertainment-books, gaming, news, celebritynewsworld, yearinoffbeatgoodnews, newstechnology, newspolitics, newsopinion, newsphotos, newsscienceandtechnology, newsgoodnews, newsus, causes-disaster-relief, newsoffbeat, newsfactcheck, newsscience, newscrime, factcheck, elections-2020-usvideo, traveltrivia, traveltripideas, voices, internationaltravel, travelnews, ustravel, travelarticle, traveltipsmusic-celebrity, music-gallery, musicnews, cma-awards, musicvideos, ads-latingrammys

\textbf{LLM:} 1. football\_ncaa

2. tennis

3. baseball\_mlb\_videos

4. soccer

5. basketball\_nba

6. outdoors

7. football\_nfl

8. football\_nfl\_videos

9. icehockey\_nhl

10. more\_sports

\end{tcolorbox}

\begin{tcolorbox}[%`colback`=gray!10,
            colframe=gray,
            width=1\linewidth,
            arc=1mm, 
            auto outer arc,
            title={Recall From Leaf Node},
            breakable,]
            \textbf{Input:} Rank top 5 news from the following candidate news about football\_ncaa to recommend to the user from the most important to the least important without explanation:
            
College football Week 12 primer: Heisman Watch, upset picks, predictions and more

Marshall marks 49th anniversary of tragic football team plane crash

Saban suspended unnamed player for Miss. St. game for not going to class

2-game suspensions for La. Tech's starting QB, star WR

No. 2 Ohio State heads to Rutgers as 51-point favorite

Opinion: Baylor football back on top four years after sexual assault scandal rocked campus

Five games in Week 12 that will impact the College Football Playoff race

Here's how Michigan State football can beat Michigan on Saturday

LSU's Ed Orgeron Is College Football's Best Head Coach Right Now | McMurphy's Law

5 young players who could lead Huskies down season's final stretch

High school football: Can Clover football continue its special run against Mauldin?

H.S. PLAYOFFS: Clemens offense in good hands with DiDomenico at the controls

Top 10 storylines for college football Week 12

SC president: Muschamp 'will be my coach through end of season'

LSU's Mighty Joe Brady is making Mickey Mouse money in the college football world

The Best Photos of College Football

Kentucky's Bowden gets Wildcats fans intrigued with tweet at Calipari

From Temple to Baylor, Matt Rhule wins in hopeless places. His secret? People skills.

A surprising 9-0, Baylor's rise to a showdown with Oklahoma was three years in the making

Bold predictions for Week 12 in college football

Archrivals Furman, Wofford meet Saturday with SoCon title hopes on the line

Notre Dame sellout streak of 273 games dating to 1973 likely to end this week against Navy

Report: Butch Jones being considered for Arkansas job

McMurphy's musings and college football picks for Week 12
            
\textbf{LLM:} 1. College football Week 12 primer: Heisman Watch, upset picks, predictions and more

2. Marshall marks 49th anniversary of tragic football team plane crash

3. Saban suspended unnamed player for Miss. St. game for not going to class

4. 2-game suspensions for La. Tech's starting QB, star WR

5. No. 2 Ohio State heads to Rutgers as 51-point favorite

\textbf{Input:} Rank top 3 news from the following candidate news about tennis to recommend to the user from the most important to the least important without explanation:

ATP Cup will be a 'great start' to year, says Becker

Zverev denies illegal phone use at ATP Finals

Andy Murray targets Australian Open after bouncing back from 'rough year'

\textbf{LLM:} 1. Andy Murray targets Australian Open after bouncing back from 'rough year'

2. ATP Cup will be a 'great start' to year, says Becker

3. Zverev denies illegal phone use at ATP Finals

\textbf{Input:} Rank top 2 news from the following candidate news about baseball\_mlb\_videos to recommend to the user from the most important to the least important without explanation:

Cody Bellinger earns NL MVP after leading LAD to 106 wins

Bud Light Ads Honor Nats Fan

\textbf{LLM:} 1. Cody Bellinger earns NL MVP after leading LAD to 106 wins

2. Bud Light Ads Honor Nats Fan

\textbf{Input:} Rank top 3 news from the following candidate news about soccer to recommend to the user from the most important to the least important without explanation:

Dest makes quick impact as US rebounds to beat Canada 4-1

Jorge Vergara, former owner of Chivas USA, dies at 64

Realio's Ratings: Seattle wins their second, this time at home

\textbf{LLM:} 1. Jorge Vergara, former owner of Chivas USA, dies at 64

2. Dest makes quick impact as US rebounds to beat Canada 4-1

3. Realio's Ratings: Seattle wins their second, this time at home
\textbf{Input:} Rank top 5 news from the following candidate news about basketball\_nba to recommend to the user from the most important to the least important without explanation:

Charania: Aron Baynes positioning himself for well over \$10 million per year in free agency

Lakers' Avery Bradley sidelined by hairline fracture in right leg; Davis expected to return

Knicks fans welcome Porzingis back with hearty round of boos

LeBron James on he and Tom Brady: 'We're gonna play until we can't walk'

Warriors on pace for worst drop in winning percentage in NBA history

Bronny James Jr. and Sierra Canyon to have 15 games streaming on ESPN

LeBron James: 'Everyone had doubt' whether an NBA team would sign Carmelo Anthony

Porzingis forgets which locker room to go to at Madison Square Garden

Hawks' Young with filthy move on Rubio

Paul felt 'stabbed in the back' by trade from Rockets

Daryl Morey wonders if MVP voters will again 'rob' James Harden

Bill Russell finally accepts Basketball Hall of Fame ring

Cam Johnson, the Suns' surprise first-round pick, is the standout among Phoenix's revamped wing rotation

Report: Carmelo Anthony returning to NBA with Trail Blazers

Solomon: Too many minutes for Rockets' Harden?

Plumlee, bench help Nuggets rally past Nets 101-93

Lakers' Avery Bradley suffers hairline fracture, to be re-evaluated in one to two weeks

Report: Knicks thought Pelicans' trade asking price for Anthony Davis was too high

NBA dynamic duos: What pairings are rocking, struggling?

Holiday's 36 points push Pelicans past Clippers 132-127

Carmelo Anthony reportedly won't debut for Portland before Tuesday, missing early Houston reunion

Same Old Clippers: Paul George Returns, Clippers Struggle, and Melo Goes to Blazers


\textbf{LLM:} 1. Charania: Aron Baynes positioning himself for well over \$10 million per year in free agency

2. Lakers' Avery Bradley sidelined by hairline fracture in right leg; Davis expected to return

3. LeBron James: 'Everyone had doubt' whether an NBA team would sign Carmelo Anthony

4. Report: Carmelo Anthony returning to NBA with Trail Blazers

5. Same Old Clippers: Paul George Returns, Clippers Struggle, and Melo Goes to Blazers

\textbf{Input:}
Rank top 1 news from the following candidate news about outdoors to recommend to the user from the most important to the least important without explanation:

2020 Barletta E24QC

\textbf{LLM:}
2020 Barletta E24QC

\textbf{Input:}
Rank top 5 news from the following candidate news about football\_nfl to recommend to the user from the most important to the least important without explanation:

Arian Foster calls out NFL fans for being hypocrites over Myles Garrett attack

Garrett will lose at least \$1.139 million

\textcolor{red}{Opinion: NFL should suspend Browns' Myles Garrett for rest of season   at minimum   for helmet swing}

Brady on Kaepernick workout: 'Pretty cool that he's getting that opportunity'

\textcolor{red}{This was uglier than a brawl. And Myles Garrett deserves suspension for rest of year after helmet attack.}

Hue Jackson will run Colin Kaepernick's passing drills, 11 teams have said they'll attend

Report: Police investigating woman's death after Redskins' player Montae Nicholson took her to hospital

Police not getting involved in Myles Garrett-Mason Rudolph incident

Maurkice Pouncey suspended three games

Freddie Kitchens: I'm embarrassed and Myles Garrett is embarrassed

Police not getting involved in Myles Garrett-Mason Rudolph incident

Belichick mocks social media in comments on Garrett incident

Sports betting: Vegas Vic's top plays are Cowboys on the road, Eagles at home and some Zach Ertz props

Colin Kaepernick heads to Atlanta for workout

New York Jets receiver Quincy Enunwa rips team, calls fines 'excessive'

Myles Garrett on attacking Mason Rudolph: 'I made a mistake, I lost my cool'

Receivers Collin Johnson, Devin Duvernay form Longhorns' most dynamic duo

Opinion: Kitchens unqualified to lead undisciplined Browns

Garrett-Rudolph fight invokes memories of other helmet incidents, Cowboys involved

Antonio Brown offers to play catch with Colin Kaepernick in private workout

Report: At least 24 teams expected to attend Kaepernick's workout

Opinion: NFL had no choice but to send a clear message with Garrett punishment

It's not just the Browns vs. Steelers. NFL has memorable history of fighting on the gridiron

Report: Rudolph won't take legal action against Garrett

Antonio Brown completes interview with NFL

Prosecuting Garrett is overkill, Rudolph got off light, Pouncey is a folk hero but he deserved 3 games

'He could have killed him:' Reaction pouring in after Browns DE hits Steelers QB with helmet

Colin Kaepernick to the Broncos? Chances aren't great, oddsmaker says.

Ex-Browns receiver Antonio Callaway gets 10-game drug ban

Browns, Steelers brawl at end of Cleveland's 21-7 win

Attorney: Garrett's actions against QB to be 'reviewed thoroughly'

Do the Broncos have a second round curse?

How Nick Williams went from being out of the NFL to leading the Bears in sacks

Wilson deletes tweet of him standing over concussed Smith-Schuster

Eagles-Patriots Week 11 Predictions: Do Birds Have Chance Against Defending Super Bowl Champs?

Mason Rudolph's agent doesn't rule out potential legal action after Myles Garrett incident

Myles Garrett, helmet a 'weapon,' banned for rest of season

NFL world stunned by Myles Garrett attack on Mason Rudolph: Calls for season-long ban, jail

Eagles' Jordan Howard not cleared for contract as Jay Ajayi visits team

Browns apologize to Mason Rudolph, call Myles Garrett's actions 'unacceptable'

Mason Rudolph: Myles Garrett's actions 'cowardly' and 'bush league'

Opinion: Colin Kaepernick is about to get what he deserves: a chance

ROAD TO THE SUPER BOWL: Portsmouth runs on Evans brothers

Matthew Stafford will not play against Cowboys with back injury

Myles Garrett bashes Mason Rudolph with helmet in Browns-Steelers fight

Police not pursuing charges against Browns' Myles Garrett

Myles Garrett issues statement apologizing for 'terrible mistake'

\textcolor{red}{Some believe Mason Rudolph, hit in head with his own helmet, isn't getting enough blame}

Baker Mayfield quick to condemn teammate Myles Garrett for brawl, attack on Mason Rudolph

Report: Myles Garrett facing lengthy suspension, could be five games

\textbf{LLM:}
1. Myles Garrett bashes Mason Rudolph with helmet in Browns-Steelers fight

2. \textcolor{red}{Opinion: NFL should suspend Browns' Myles Garrett for rest of season at minimum for helmet swing}

3. Myles Garrett, helmet a 'weapon,' banned for rest of season

4. Baker Mayfield quick to condemn teammate Myles Garrett for brawl, attack on Mason Rudolph

5. \textcolor{red}{Some believe Mason Rudolph, hit in head with his own helmet, isn't getting enough blame}


\end{tcolorbox}

\begin{tcolorbox}[%`colback`=gray!10,
            colframe=gray,
            width=1\linewidth,
            arc=1mm, 
            auto outer arc,
            title={Diversity-aware Re-rank},
            breakable,]
            \textbf{Input:}
            Rank these pre-selected news based on user interests. Be aware of ranking diversity.
            
1: College football Week 12 primer: Heisman Watch, upset picks, predictions and more

2: Marshall marks 49th anniversary of tragic football team plane crash

3: Saban suspended unnamed player for Miss. St. game for not going to class

4: 2-game suspensions for La. Tech's starting QB, star WR

5: No. 2 Ohio State heads to Rutgers as 51-point favorite

6: Andy Murray targets Australian Open after bouncing back from 'rough year'

7: ATP Cup will be a 'great start' to year, says Becker

8: Zverev denies illegal phone use at ATP Finals

9: Cody Bellinger earns NL MVP after leading LAD to 106 wins

10: Bud Light Ads Honor Nats Fan

11: Jorge Vergara, former owner of Chivas USA, dies at 64

12: Dest makes quick impact as US rebounds to beat Canada 4-1

13: Realio's Ratings: Seattle wins their second, this time at home

14: Charania: Aron Baynes positioning himself for well over \$10 million per year in free agency

15: Lakers' Avery Bradley sidelined by hairline fracture in right leg; Davis expected to return

16: LeBron James: 'Everyone had doubt' whether an NBA team would sign Carmelo Anthony

17: Report: Carmelo Anthony returning to NBA with Trail Blazers

18: Same Old Clippers: Paul George Returns, Clippers Struggle, and Melo Goes to Blazers

19: 2020 Barletta E24QC

\textcolor{red}{20: Opinion: NFL should suspend Browns' Myles Garrett for rest of season at minimum for helmet swing}

21: Myles Garrett bashes Mason Rudolph with helmet in Browns-Steelers fight

22: Myles Garrett, helmet a 'weapon,' banned for rest of season

23: Baker Mayfield quick to condemn teammate Myles Garrett for brawl, attack on Mason Rudolph

\textcolor{red}{24: Some believe Mason Rudolph, hit in head with his own helmet, isn't getting enough blame}
            
\textbf{LLM:} Based on user interests and ranking diversity, the pre-selected news can be ranked as follows:

1. Andy Murray targets Australian Open after bouncing back from 'rough year'

2. Dest makes quick impact as US rebounds to beat Canada 4-1

3. Cody Bellinger earns NL MVP after leading LAD to 106 wins

4. LeBron James: 'Everyone had doubt' whether an NBA team would sign Carmelo Anthony

5. Report: Carmelo Anthony returning to NBA with Trail Blazers

6. Lakers' Avery Bradley sidelined by hairline fracture in right leg; Davis expected to return

7. Same Old Clippers: Paul George Returns, Clippers Struggle, and Melo Goes to Blazers

\textcolor{red}{8. Opinion: NFL should suspend Browns' Myles Garrett for rest of season at minimum for helmet swing}

9. Myles Garrett, helmet a 'weapon,' banned for rest of season

10. Baker Mayfield quick to condemn teammate Myles Garrett for brawl, attack on Mason Rudolph

\textcolor{red}{11. Some believe Mason Rudolph, hit in head with his own helmet, isn't getting enough blame}

12. Myles Garrett bashes Mason Rudolph with helmet in Browns-Steelers fight

13. College football Week 12 primer: Heisman Watch, upset picks, predictions and more

14. Marshall marks 49th anniversary of tragic football team plane crash

15. Saban suspended unnamed player for Miss. St. game for not going to class

16. 2-game suspensions for La. Tech's starting QB, star WR

17. No. 2 Ohio State heads to Rutgers as 51-point favorite

18. ATP Cup will be a 'great start' to year, says Becker

19. Zverev denies illegal phone use at ATP Finals

20. Charania: Aron Baynes positioning himself for well over \$10 million per year in free agency

21. Bud Light Ads Honor Nats Fan

22. Jorge Vergara, former owner of Chivas USA, dies at 64

23. Realio's Ratings: Seattle wins their second, this time at home

24. 2020 Barletta E24QC

Please note that this ranking is subjective and can vary based on individual interests and preferences.
\\
\end{tcolorbox}

% ################################
% Evaluation
% ################################
% Ground Truth News:
% 	 Some believe Mason Rudolph, hit in head with his own helmet, isn't getting enough blame
% 	 Opinion: NFL should suspend Browns' Myles Garrett for rest of season   at minimum   for helmet swing
% 	 This was uglier than a brawl. And Myles Garrett deserves suspension for rest of year after helmet attack.

% Success recall news: 
% 	 Opinion: NFL should suspend Browns' Myles Garrett for rest of season   at minimum   for helmet swing
% 	 Some believe Mason Rudolph, hit in head with his own helmet, isn't getting enough blame

% ################################
